# Supplementary material for: Diffusion-Based Image-to-Image Translation by Noise Correction via Prompt Interpolation
Source: arXiv:2409.08077 source file (2024-09-12)
Supplement: Supplementary file 1 [file X_suppl.tex]

% \clearpage
% \setcounter{page}{1}
%\maketitle
%\\supplementary

\section{Supplementary Material}

\subsection{Ablation Study}

We proposed our algorithm PIC in this paper. 
Two main points of PIC are 'Noise Correction (NC)' and '(Smooth) Prompt Interpolation (PI)'. 
In this section, we report both quantitative and qualitative results to verify performance in I2I Translation gets better when using two main points. We compare 4 algorithms in this section.: "(na\"ive) DDIM", "DDIM + NC", "DDIM + PI", "DDIM + NC + PI (Ours)". We used same experimental setting in main paper.

\subsubsection{Quantitative Results}

\begin{figure*}[t!]
	\centering
	%\vspace{-5pt}
	%\vspace{0.2cm}
	\includegraphics[width=1.0\linewidth]{../figures/CVPR_Supplementary_Ablation.pdf}
	%\vspace{-5pt}
	\caption{Ablation Study.}
	%Qualitative comparisons between the proposed method and state-of-the-art methods~\cite{hertz2023prompt, tumanyan2023plug, parmar2023zero} on real images sampled from the LAION-5B dataset~\cite{schuhmann2022laion} using the pretrained Stable Diffusion~\cite{rombach2022high}.}
%Qualitative results of Pix2Pix on the Cityscapes dataset.
% ``Output" denotes the ground-truth and ``Original" represents the uncompressed generator.}
%\vspace{0.3cm}
\label{fig:ablation_ours}
\end{figure*}

Our comparison results are shown in Table \red{5}. 
\subsection{Additional Comparison}

\begin{table}[t!]
	\centering
	\caption{
		%and real images sampled from the LAION-5B dataset~\citep{schuhmann2022laion} for various tasks.
		%  text-driven image-to-image translation methods~\citep{hertz2022prompt, tumanyan2023plug, parmar2023zero} using the pre-trained Stable Diffusion~\citep{rombach2022high} and real images sampled from LAION 5B dataset~\citep{schuhmann2022laion} for various tasks. 
		%
		% For the the drawing $\rightarrow$ oil painting task, we do not report the BD score since the background can not be clearly defined.
		%and the lower value does not imply that the algorithm achieves good performance.
		Black and red bold-faced numbers represent the best and second-best performances for each metric in each row. 
	}
	%\vspace{0.1in}
	\setlength\tabcolsep{6pt} 
	\scalebox{0.80}{
		%\resizebox{\linewidth}{!}{
			\hspace{-2mm}
			\begin{tabular}{l ccc | ccc | ccc | ccc}
				%\begin{tabular}{l ccc ccc ccc ccc ccc}
				%\toprule 
				\hline
				\multirow{2}{*}{Task} 
				%& \multicolumn{3}{c}{DDIM}
				& \multicolumn{3}{c|}{DDIM}
				& \multicolumn{3}{c|}{DDIM+PI}
				& \multicolumn{3}{c|}{DDIM+NC} 
				& \multicolumn{3}{c}{DDIM+PI+NC(Ours)} \\ 
				%& \multicolumn{3}{c}{Avg} \\ %\\
				
				\cline{2-4} \cline{5-7} \cline{8-10} \cline{11-13}
				%\cline{2-4} \cline{5-7} \cline{8-10} \cline{11-13} \cline{14-16}
				& CS ($\uparrow$)
				& BD ($\downarrow$)
				& SD ($\downarrow$)

				& CS ($\uparrow$)
				& BD ($\downarrow$)
				& SD ($\downarrow$)
				
				& CS ($\uparrow$)
				& BD ($\downarrow$)
				& SD ($\downarrow$)

				& CS ($\uparrow$)
				& BD ($\downarrow$)
				& SD ($\downarrow$)
				
				%& CS ($\uparrow$)
				%& BD ($\downarrow$)
				%& SD ($\downarrow$)
				
				\\ 
				\cline{1-13}
				%\cline{1-16}
				
				{dog $\rightarrow$ cat}
				% & ? & ? & ?
				& \bred{0.289} & 0.158 & 0.086 
				& \bred{0.289} & 0.130 & 0.070
				& \black{0.293} & \bred{0.054} & \bred{0.038}
				& \black{0.293} & \black{0.045} & \black{0.031} \\
				%& \black{0.293} & \black{0.045} & \black{0.031}\\

				{cat $\rightarrow$ dog}
				% & ? & ? & ?
				& 0.283 & 0.185 & 0.089
				& \bred{0.285} & 0.150 & 0.070
				& \black{0.288} & \bred{0.068} & \bred{0.041}
				& \black{0.288} & \black{0.057} & \black{0.033} \\
				%& \black{0.293} & \black{0.045} & \black{0.031}\\

				{horse $\rightarrow$ zebra}
				% & ? & ? & ?
				& 0.325	& 0.287	& 0.123
				& \bred{0.330}	& 0.214	& 0.097
				& \black{0.333}	& \bred{0.113}	& \bred{0.050}
				& 0.324	& \black{0.085}	& \black{0.037} \\
				%& \black{0.293} & \black{0.045} & \black{0.031}\\

				{zebra $\rightarrow$ horse}
				% & ? & ? & ?
				& \black{0.294}	& 0.295	& 0.104
				& \black{0.294}	& 0.254	& 0.097
				& \black{0.294}	& \bred{0.139}	& \bred{0.055}
				& \bred{0.292}	& \black{0.126}	& \black{0.050} \\
				%& \black{0.293} & \black{0.045} & \black{0.031}\\

				{tree $\rightarrow$ palm tree}
				& 0.304	& 0.234	& 0.088
				& 0.306 & \bred{0.222}	& 0.084
				& \bred{0.312} & \black{0.085}	& \bred{0.056}
				& \black{0.314}	& \black{0.085}	& \black{0.036} \\
				% & \black{0.293} & \black{0.045} & \black{0.031}\\
				
				{dog $\rightarrow$ dog w/ glasses}
				& \black{0.318}	& 0.134	& 0.072
				& 0.310	& 0.132	& 0.065 
				& \bred{0.317}	& \bred{0.029}	& \bred{0.021}
				& 0.312	& \black{0.026}	& \black{0.016} \\
				%& \black{0.293} & \black{0.045} & \black{0.031} \\

				\hline
				{Average}
				& 0.302	& \bred{0.113}	& 0.040
				& \black{0.305}	& 0.120	& \bred{0.036} 
				& 0.301	& 0.136	& 0.066 
				& \bred{0.304}	& \black{0.071}	& \black{0.034} \\
				%& \black{0.293} & \black{0.045} & \black{0.031} \\
				
				\hline
				%\bottomrule 
			\end{tabular}
			
			%}
	}
	\label{tab:ablation}
\end{table}

\subsection{Inference Time}

\begin{figure*}[t!]
	\centering
	%\vspace{-5pt}
	%\vspace{0.2cm}
	\includegraphics[width=1.0\linewidth]{../figures/CVPR_Supplementary_Comparison1.pdf}
	%\vspace{-5pt}
	\caption{Image translation results using the proposed method on data sampled from the LAION-5B dataset~\cite{schuhmann2022laion}. The proposed method effectively preserves the structure or the background of the source image while successfully editing the region of interest.}
	%Qualitative comparisons between the proposed method and state-of-the-art methods~\cite{hertz2023prompt, tumanyan2023plug, parmar2023zero} on real images sampled from the LAION-5B dataset~\cite{schuhmann2022laion} using the pretrained Stable Diffusion~\cite{rombach2022high}.}
%Qualitative results of Pix2Pix on the Cityscapes dataset.
% ``Output" denotes the ground-truth and ``Original" represents the uncompressed generator.}
%\vspace{0.3cm}
\label{fig:visualization_ours}
\end{figure*}

\begin{figure*}[t!]
	\centering
	%\vspace{-5pt}
	%\vspace{0.2cm}
	\includegraphics[width=1.0\linewidth]{../figures/CVPR_Supplementary_Comparison2.pdf}
	%\vspace{-5pt}
	\caption{Image translation results using the proposed method on data sampled from the LAION-5B dataset~\cite{schuhmann2022laion}. The proposed method effectively preserves the structure or the background of the source image while successfully editing the region of interest.}
	%Qualitative comparisons between the proposed method and state-of-the-art methods~\cite{hertz2023prompt, tumanyan2023plug, parmar2023zero} on real images sampled from the LAION-5B dataset~\cite{schuhmann2022laion} using the pretrained Stable Diffusion~\cite{rombach2022high}.}
%Qualitative results of Pix2Pix on the Cityscapes dataset.
% ``Output" denotes the ground-truth and ``Original" represents the uncompressed generator.}
%\vspace{0.3cm}
\label{fig:visualization_ours}
\end{figure*}

\begin{figure*}[t!]
	\centering
	%\vspace{-5pt}
	%\vspace{0.2cm}
	\includegraphics[width=1.0\linewidth]{../figures/CVPR_Supplementary_Visualization.pdf}
	%\vspace{-5pt}
	\caption{Visualization of noise correction in I2I Translations.}
	%Qualitative comparisons between the proposed method and state-of-the-art methods~\cite{hertz2023prompt, tumanyan2023plug, parmar2023zero} on real images sampled from the LAION-5B dataset~\cite{schuhmann2022laion} using the pretrained Stable Diffusion~\cite{rombach2022high}.}
%Qualitative results of Pix2Pix on the Cityscapes dataset.
% ``Output" denotes the ground-truth and ``Original" represents the uncompressed generator.}
%\vspace{0.3cm}
\label{fig:visualization_ours}
\end{figure*}

\begin{figure*}[t!]
	\centering
	%\vspace{-5pt}
	%\vspace{0.2cm}
	\includegraphics[width=1.0\linewidth]{../figures/CVPR_Supplementary_AFHQ.pdf}
	%\vspace{-5pt}
	\caption{Image translation results using the proposed method on data sampled from the AFHQ Dataset.}
	%Qualitative comparisons between the proposed method and state-of-the-art methods~\cite{hertz2023prompt, tumanyan2023plug, parmar2023zero} on real images sampled from the LAION-5B dataset~\cite{schuhmann2022laion} using the pretrained Stable Diffusion~\cite{rombach2022high}.}
%Qualitative results of Pix2Pix on the Cityscapes dataset.
% ``Output" denotes the ground-truth and ``Original" represents the uncompressed generator.}
%\vspace{0.3cm}
\label{fig:visualization_ours}
\end{figure*}

% \section{Rationale}
% \label{sec:rationale}
% % 
% Having the supplementary compiled together with the main paper means that:
% % 
% \begin{itemize}
 %\item The supplementary can back-reference sections of the main paper, for example, we can refer to % \cref{sec:intro};
% \item The main paper can forward reference sub-sections within the supplementary explicitly (e.g. % referring to a particular experiment); 
% \item When submitted to arXiv, the supplementary will already included at the end of the paper.
% \end{itemize}
% 
% To split the supplementary pages from the main paper, you can use \href{https://support.apple.com/en-ca/guide/preview/prvw11793/mac#:~:text=Delete%20a%20page%20from%20a,or%20choose%20Edit%20%3E%20Delete).}{Preview (on macOS)}, \href{https://www.adobe.com/acrobat/how-to/delete-pages-from-pdf.html#:~:text=Choose%20%E2%80%9CTools%E2%80%9D%20%3E%20%E2%80%9COrganize,or%20pages%20from%20the%20file.}{Adobe Acrobat} (on all OSs), as well as \href{https://superuser.com/questions/517986/is-it-possible-to-delete-some-pages-of-a-pdf-document}{command line tools}.
